# Supplementary material for: A smart electric bike for smart cities
Source: arXiv:2203.06679 source file (2022-03-13)
Supplement: Supplementary file 1 [file appendix-1.tex]

%\chapter*{Appendix A}
%
%From system design->Hardware-> data transfer
%
%This PWM signal had to be converted to an analog voltage which is the required control input to the main Grinfineon controller of the bike. This conversion was done using a low-pass RC filter as shown in Figure \ref{fig:circuit_schematic}. The Resistor value ($\Omega$) and Capacitor value (Farads) had to be chosen based on the 
%
%%http://sim.okawa-denshi.jp/en/PWMtool.php
%
%The relationship between $V_{out}$ and $V_{in}$ is:
%\begin{equation*}
%V_{out} = \biggr(\frac{1}{1+j\omega RC}\biggr)V_{in}
%\end{equation*}
%Which yields the transfer function as:
%\begin{equation*}
%H(s) = \biggr|\frac{1}{1+\omega^2 R^2C^2}\biggr|
%\end{equation*}
%Which has a single pole at:
%\begin{equation*}
%p_1 = -\frac{1}{RC}
%\end{equation*}
%The PWM carrier frequency output from the arduino pin was 488Hz. For the PWM signal to be converted to an analog signal
%\begin{equation*}
%Analog voltage = A \times Duty Cycle
%\end{equation*}
%Where the duty cycle is the time
%\begin{equation*}
%\frac{T_{ON}}{T_{ON}+T_{OFF}}
%\end{equation*}
%In the frequency domain a low-pass filter suppresses high frequency components of an input signal and the time domain equivalent of this effect is averaging, thus by low-pass filtering a PWM signal we are extracting its average value.\\
%https://www.allaboutcircuits.com/technical-articles/turn-your-pwm-into-a-dac/ \\
%As such, the resistor and capacitor values were selected to be $R=5k\Omega$ and $C=10 \mu F$.\\
%
%
%ADD TRANSFER FUNCTION and basis for choosing R and C	\\
%ADD: Graph of PWM input vs output analog voltage\\
%ADD: Talk about resolution of PWM?\\
%Question:\\
%How does a low pass RC filter work? / How does a low pass RC filter block high frequency components of a signal?\\
%
%RC filter / PWM to Analog - graph showing translation between PWM value and analog voltage?\\
%Arduino - PWM output frequency\\
%PCB / shield, voltage regulator \\
%Comms protocols - Bluetooth,serial comms \\
%
%
